# Supplementary material for: Brownian magneto-gyrator as a tunable microengine
Source: arXiv:2110.05284 source file (2021-10-11)
Supplement: Supplementary file 1 [file Supplementalmaterials.pdf]

# Supplemental Materials: Brownian magneto-gyrator as a tunable microengine

**Iman Abdoli[1], René Wittmann[2], Joseph Michael Brader[3], Jens-Uwe Sommer[1,4], Hartmut Löwen[2], and Abhinav Sharma[1,4,*]**

[1]Leibniz-Institut für Polymerforschung Dresden, Institut Theorie der Polymere, Dresden, 01069, Germany
[2]Institut für Theoretische Physik II, Weiche Materie, Heinrich-Heine-Universität Düsseldorf, Düsseldorf, 40225, Germany
[3]Department de Physique, Université de Fribourg, CH-1700 Fribourg, Switzerland
[4]Technische Universität Dresden, Institut für Theoretische Physik, Dresden, 01069, Germany
[*]sharma@ipfdd.de

## Low-mass limit of Langevin equation

In the presence of a magnetic field, the overdamped Langevin equation can not be derived by setting the inertial term to zero. Anomalous fluxes has been observed in overdamped Brownian dynamics by setting the inertial term to zero in the velocity Langevin equation due to Lorentz force[1]. Here we take the low-mass approach[2] to derive the overdamped Langevin equation describing the dynamics of the Brownian gyrator. The velocity Langevin equation for the position $\boldsymbol{r} = (x,y)^\top$ and the velocity $\boldsymbol{v} = (v_x, v_y)$ of a particle of mass $m$ and charge $q$, subjected to a magnetic field $B$ in the $\hat{z}$ direction, can be written as

$$m\dot{\boldsymbol{v}} = \boldsymbol{F}(\boldsymbol{r}(t)) - \boldsymbol{G}\boldsymbol{v}(t) + \boldsymbol{\xi}(t), \tag{1}$$

where $\boldsymbol{F}(\boldsymbol{r}) = (F_x(\boldsymbol{r}), F_y(\boldsymbol{r}))^\top$ is the external force and $\boldsymbol{\xi}(t) = (\xi_x(t), \xi_y(t))^\top$ is the Gaussian white noise with zero mean and Dirac delta correlation $\langle \boldsymbol{\xi}(t)\boldsymbol{\xi}^\top(t')\rangle = 2\gamma \mathrm{T}\delta(t-t')$ with $\gamma$ being the friction coefficient and $\mathrm{T} = \boldsymbol{diag}(T_c, T_h)$. The matrix $\boldsymbol{G}$ is defined as

$$\boldsymbol{G} = \gamma \begin{pmatrix} 1 & -\kappa \\ \kappa & 1 \end{pmatrix}, \tag{2}$$

with $\kappa = qB/\gamma$ being the diffusive Hall parameter which quantifies the strength of the Lorentz force relative to the frictional force. By omitting the transient term $e^{-\boldsymbol{G}t/m}\boldsymbol{v}(0)$, which is negligible in the low-mass limit, the formal solution to Eq. (1) can be written as

$$\boldsymbol{v}(t) = \frac{1}{m}\int_0^t \mathrm{d}t' e^{-\frac{\boldsymbol{G}}{m}(t-t')}[\boldsymbol{F}(\boldsymbol{r}(t')) + \boldsymbol{\xi}(t')]. \tag{3}$$

which yields the following stochastic integrodifferntial equation

$$\dot{\boldsymbol{r}}(t) = \frac{1}{m}\int_0^t \mathrm{d}t' e^{-\frac{\boldsymbol{G}}{m}(t-t')}\boldsymbol{F}(\boldsymbol{r}(t')) + \boldsymbol{\chi}_m(t), \tag{4}$$

where $\boldsymbol{\chi}_m(t)$ is Gaussian non-white noise given as

$$\boldsymbol{\chi}_m(t) = \frac{1}{m}\int_0^t \mathrm{d}t' e^{-\frac{\boldsymbol{G}}{m}(t-t')}\boldsymbol{\xi}(t'). \tag{5}$$

The main purpose of this section is to derive the statistical properties of this noise and thereby the overdamped Langevin equation. From Eq. (5) it is clear that the first moment of the noise is zero, i.e., $\langle \boldsymbol{\chi}_m(t)\rangle = 0$. The interesting property of the noise is encoded in its time correlation $\langle \boldsymbol{\chi}_m(t)\boldsymbol{\chi}_m^\top(s)\rangle = \boldsymbol{\Sigma}_m(t,s)$ in the low-mass limit. Here $\boldsymbol{\Sigma}_m(t,s)$ is the correlation matrix and the subscript indicates the mass dependence of the quantity. The correlation matrix can be written as

$$\boldsymbol{\Sigma}_m(t,s) = \frac{1}{m^2}\int_0^s \mathrm{d}u \int_0^t \mathrm{d}t' e^{-\frac{\boldsymbol{G}}{m}(t-t')}\langle \boldsymbol{\xi}(t')\boldsymbol{\xi}^\top(u)\rangle e^{-\frac{\boldsymbol{G}^\top}{m}(s-u)}, \tag{6}$$

where using the properties of the Gaussian white noise $\boldsymbol{\xi}(t)$, in the limit that $t \to \infty$ and $s \to \infty$ and for a finite $t-s$, it can be rewritten as

$$\boldsymbol{\Sigma}_m(t,s) = \frac{2\gamma}{m^2} e^{-\frac{\boldsymbol{G}}{m}(t-s)} \lim_{s\to\infty} \int_0^s \mathrm{d}u \left[ e^{-\frac{\boldsymbol{G}}{m}(s-u)} \mathrm{T} e^{-\frac{\boldsymbol{G}^\top}{m}(s-u)} \right], \tag{7}$$

if $t \geq s$ and

$$\boldsymbol{\Sigma}_m(t,s) = \frac{2\gamma}{m^2} \left[ \lim_{t\to\infty} \int_0^t \mathrm{d}t' e^{-\frac{\boldsymbol{G}}{m}(t-t')} \mathrm{T} e^{\frac{-\boldsymbol{G}^\top}{m}(t-t')} \right] e^{-\frac{\boldsymbol{G}^\top}{m}(s-t)}, \tag{8}$$

if $t < s$. The integrals in Eq. (7) and Eq. (8) can be easily calculated, which yield

$$\boldsymbol{\Sigma}_m(t,s) = \begin{cases} \frac{1}{m} e^{-\frac{\boldsymbol{G}}{m}(t-s)} \boldsymbol{C}, & t \geq s, \\ \frac{1}{m} \boldsymbol{C} e^{-\frac{\boldsymbol{G}^\top}{m}(s-t)}, & t < s. \end{cases} \tag{9}$$

where the matrix $\boldsymbol{C}$ is defined as

$$\boldsymbol{C} = \frac{1}{2(1+\kappa^2)} \begin{pmatrix} 2T_c + \kappa^2(T_c+T_h) & \kappa(T_h - T_c) \\ \kappa(T_h - T_c) & 2T_h + \kappa^2(T_c+T_h) \end{pmatrix}. \tag{10}$$

The correlation matrix $\boldsymbol{\Sigma}_m$ depends on $s' \equiv t-s$ and satisfies $\boldsymbol{\Sigma}_m(-s') = \boldsymbol{\Sigma}_m^\top(s')$. The elements of the correlation functions are given by

$$\boldsymbol{\Sigma}_m(s') = \frac{1}{m} \boldsymbol{C}^{1-a} e^{-\frac{\gamma}{m}|s'|} \begin{pmatrix} \cos\left(\frac{qB}{m}s'\right) & \sin\left(\frac{qB}{m}s'\right) \\ -\sin\left(\frac{qB}{m}s'\right) & \cos\left(\frac{qB}{m}s'\right) \end{pmatrix} \boldsymbol{C}^a. \tag{11}$$

where $a = 0$ if $s' < 0$ and $a = 1$ otherwise. As $m$ decreases, the correlation functions become singular with diverging oscillation frequency $qB/m$, diverging amplitude proportional to $1/m$, and vanishing decay time $m/\gamma$. It can be shown that for any function $h(s')$ with no singularity around $s' = 0$, the low-mass limit yields

$$\lim_{m\to 0} \int_0^\infty \mathrm{d}s'\, h(s') \boldsymbol{\Sigma}_m(s') = h(0) \boldsymbol{G}^{-1} \boldsymbol{C}, \tag{12}$$

$$\lim_{m\to 0} \int_{-\infty}^0 \mathrm{d}s'\, h(s') \boldsymbol{\Sigma}_m(s') = h(0) \boldsymbol{C} (\boldsymbol{G}^{-1})^\top. \tag{13}$$

Therefore, the correlation matrix in the low-mass limit, i.e., $m \to 0$ can be written as

$$\boldsymbol{\Sigma}(s') \equiv \lim_{m\to 0} \boldsymbol{\Sigma}_m(s') = \boldsymbol{G}^{-1} \boldsymbol{C} \delta_+(s') + \boldsymbol{C} (\boldsymbol{G}^{-1})^\top \delta_-(s'), \tag{14}$$

where the notations $\delta_\pm(s')$ indicate the different Dirac delta functions which are zero for $s' \neq 0$ while $\int_0^\infty \mathrm{d}s' \delta_+(s') = \int_{-\infty}^0 \mathrm{d}s' \delta_-(s') = 1$ and $\int_0^\infty \mathrm{d}s' \delta_-(s') = \int_{-\infty}^0 \mathrm{d}s' \delta_+(s') = 0$.

To complete the derivation of the overdamped Langevin equation we now evaluate the first term on the right hand side of Eq. (4). Using the change of variable from $t'$ to $s' = t - t'$ it can be written as

$$\frac{1}{m} \int_0^t \mathrm{d}t' e^{-\frac{\boldsymbol{G}}{m}(t-t')} \boldsymbol{F}(\boldsymbol{r}(t')) = \left[ \int_0^t \mathrm{d}s'\, \boldsymbol{\Sigma}_m(s') \boldsymbol{F}(\boldsymbol{r}(t-s')) \right] \boldsymbol{C}^{-1}, \tag{15}$$

where using Eq. (12), in the low-mass limit converges to $\boldsymbol{G}^{-1}\boldsymbol{F}(\boldsymbol{r}(t))$. Thus the Langevin equation in the low-mass limit corresponding to the overdamped dynamics can be written as

$$\dot{\boldsymbol{r}}(t) = \boldsymbol{G}^{-1} \boldsymbol{F}(\boldsymbol{r}(t)) + \boldsymbol{\chi}(t), \tag{16}$$

where $\boldsymbol{\chi}(t)$ is Gaussian non-white noise with zero mean and the time correlation as in Eq. (14).

## Efficiency of a Brownian magneto-gyrator

The exchange of energy between a Brownian particle and its surrounding environment becomes stochastic at the microscale and yet work, heat, and efficiency can be defined through the framework of stochastic thermodynamics[3]. In this section, we aim to determine such quantities. The Langevin equation (1) for the particle under a load of the form of the nonconservative force $\boldsymbol{F}_{nc} = \varepsilon(y, -x)$ with the parameter $\varepsilon$ and in the harmonic potential $\mathrm{V}(x, y) = k(x^2 + \alpha y^2)/2$ can be rewritten as

$$\dot{\boldsymbol{z}}(t) = -\boldsymbol{F}\boldsymbol{z}(t) + \tilde{\boldsymbol{\xi}}(t), \tag{17}$$

where $\boldsymbol{z}(t) = (x(t), y(t), v_x(t), v_y(t))^\top$ and $\tilde{\boldsymbol{\xi}}(t) = (0, 0, m^{-1}\xi_x(t), m^{-1}\xi_y(t))^\top$ is Gaussian white noise with zero mean and time correlation $\langle \tilde{\boldsymbol{\xi}}(t)\tilde{\boldsymbol{\xi}}^\top(t')\rangle = (2\gamma/m^2)\mathrm{T}\delta(t-t')$ where $\gamma$ is the constant friction coefficient. Here $k$ is the stiffness of the potential, $\alpha$ is a dimensionless parameter, and $\mathrm{T} = \boldsymbol{diag}(0, 0, T_c, T_h)$ is a diagonal matrix. Note that T is a two-dimensional matrix in Eq. (1). The matrix $\boldsymbol{F}$ is defined as

$$\boldsymbol{F} = \frac{1}{m}\begin{pmatrix} \boldsymbol{0} & -m\mathbb{I} \\ \mathrm{U}_l & \boldsymbol{G} \end{pmatrix}, \tag{18}$$

where $\mathbb{I}$ is the identity matrix and

$$\boldsymbol{G} = \gamma\begin{pmatrix} 1 & -\kappa \\ \kappa & 1 \end{pmatrix}, \qquad \mathrm{U}_l = k\begin{pmatrix} 1 & -\varepsilon' \\ \varepsilon' & \alpha \end{pmatrix}. \tag{19}$$

where $\varepsilon' = \varepsilon/k$ is a dimensionless parameter. In order to calculate the efficiency of the microengine the calculation of the rate of the heat loss, $\langle \dot{Q}\rangle$ and the average mechanical power, $P$ is needed, which can be determined by the steady-state covariance matrix $\mathrm{S} = \lim_{t\to\infty}\mathrm{S}(t)$, where $\mathrm{S}(t) = \langle \boldsymbol{z}(t)\boldsymbol{z}^\top(t)\rangle$. The change in the covariance matrix in the time interval $\mathrm{d}t$ is given by

$$\mathrm{dS}(t) = -[\boldsymbol{F}\mathrm{S}(t) + \mathrm{S}(t)\boldsymbol{F}^\top]\,\mathrm{d}t + \int_t^{t+\mathrm{d}t}\mathrm{d}t'\int_t^{t+\mathrm{d}t}\mathrm{d}t''\langle\tilde{\boldsymbol{\xi}}(t')\tilde{\boldsymbol{\xi}}^\top(t'')\rangle, \tag{20}$$

which using the property of the noise $\tilde{\boldsymbol{\xi}}$, the time evolution of the covariance matrix can be written as

$$\frac{\mathrm{dS}(t)}{\mathrm{d}t} = -\boldsymbol{F}\mathrm{S}(t) - \mathrm{S}(t)\boldsymbol{F}^\top + \frac{2\gamma}{m^2}\mathrm{T}. \tag{21}$$

The steady-state covariance matrix can be calculated by setting $\mathrm{dS}(t)/\mathrm{d}t$ to zero, which consists of the steady-state position-position, position- and velocity-velocity correlations. The solution to Eq. (21) gives the steady-state covarinace matrix with the following elements

$$\begin{aligned}
\langle x^2\rangle &= \frac{[(\alpha - \alpha^2 + \varepsilon'^2)(1 - \alpha - 2\varepsilon'\kappa) - 2\alpha\varepsilon'^2]M + 2[\varepsilon'^2 + (1+\kappa^2)\alpha^2 + \alpha]}{S_0 k(\varepsilon'^2 + \alpha)}T_c \\
&+ \frac{\varepsilon'^2(1 + \alpha + 2\varepsilon'\kappa)M + 2(1+\kappa^2)\varepsilon'^2 + 2\alpha\kappa^2}{S_0 k(\varepsilon'^2 + \alpha)}T_h, && (22)\\
\langle y^2\rangle &= \frac{\varepsilon'^2(1 + \alpha + 2\varepsilon'\kappa)M + (1+\kappa^2)\varepsilon'^2 + \alpha\kappa^2}{S_0 k(\varepsilon'^2 + \alpha)}T_c \\
&+ \frac{[(1-\alpha^2) - \varepsilon'(1-\alpha)(\varepsilon' - 2\varepsilon'\kappa) - 2\varepsilon'^2(1 + \varepsilon'\kappa)]M + 2(1 + \alpha + \varepsilon'^2 + \kappa^2)}{S_0 k(\varepsilon'^2 + \alpha)}T_h, && (23)\\
\langle v_x^2\rangle &= k\frac{[(\alpha-1)^2 - 2\varepsilon'(\varepsilon' + (1-\alpha)\kappa)]M + (2+\kappa^2)(1 + \alpha - 2\varepsilon'\kappa)}{\gamma^2 M S_0}T_c + k\frac{\kappa^2(1 + \alpha - 2\varepsilon'\kappa) + 2\varepsilon'^2 M}{\gamma^2 M S_0}T_h, && (24)\\
\langle v_y^2\rangle &= k\frac{\kappa^2(1 + \alpha - 2\varepsilon'\kappa) + 2\varepsilon'^2 M}{\gamma^2 M S_0}T_c + k\frac{[(\alpha-1)^2 - 2\varepsilon'(\varepsilon' - (1-\alpha)\kappa)]M + (2+\kappa^2)(1 + \alpha - 2\varepsilon'\kappa)}{\gamma^2 M S_0}T_h, && (25)\\
& && (26)
\end{aligned}$$

where $M = km/\gamma^2$ is a dimensionless parameter and the non-diagonal elements are given as

$$\begin{aligned}
\langle xy\rangle &= \frac{[\alpha(\alpha-1+2\varepsilon'\kappa)-2\varepsilon'^2]\varepsilon' M+2[\alpha(\varepsilon'-\kappa+\varepsilon'\kappa^2)-\varepsilon'^2]}{S_0 k(\varepsilon'^2+\alpha)}T_c \\
&+ \frac{(2\varepsilon'^2+\alpha-1-2\varepsilon'\kappa)\varepsilon' M+2[\kappa(\alpha+\varepsilon'^2)-\varepsilon'(1+\kappa^2)]}{S_0 k(+\varepsilon'^2+\alpha)}T_h, && (27)\\
\langle yx\rangle &= \langle xy\rangle, && (28)\\
\langle xv_x\rangle &= \langle v_x x\rangle = 0, && (29)\\
\langle yv_y\rangle &= \langle v_y y\rangle = 0, && (30)\\
\langle xv_y\rangle &= \frac{\kappa(1-\alpha)(T_h-T_c)+2\varepsilon'(1+\kappa^2)(T_c+T_h)}{S_0}, && (31)\\
\langle v_y x\rangle &= \langle xv_y\rangle, && (32)\\
\langle yv_x\rangle &= -\langle xv_y\rangle, && (33)\\
\langle v_x y\rangle &= \langle yv_x\rangle, && (34)\\
\langle v_x v_y\rangle &= k\frac{[(\alpha-1)(T_c+T_h)-2\kappa\varepsilon'^2(T_h-T_c)]\varepsilon' M+\kappa(1+\alpha-2\varepsilon'\kappa)(T_h-T_c)}{\gamma^2 M S_0}, && (35)\\
\langle v_y v_x\rangle &= \langle v_x v_y\rangle, && (36)\\
& && (37)
\end{aligned}$$

where $S_0 = [(\alpha-1)^2 - 4\varepsilon'^2(1+\kappa^2)]M + 2(1+\kappa^2)(1+\alpha-2\varepsilon'\kappa)$. Note that taking the small-mass limit of the covariance matrix gives the correlations in the overdamped regime. Since we finally need the kinetic energy of the particle which is proportional to $M(\langle v_x^2\rangle + \langle v_y^2\rangle)$, in the overdamped regime the small-mass limit of $M\langle v_x^2\rangle$ and $M\langle v_y^2\rangle$ is required which makes Eq. (24) and Eq. (25) well-defined. However, for the cross-correlation in Eq. (35) the explicit knowledge of the particle's mass is needed even in the overdamped limit.

The efficiency is given by the ratio between the extracted work and the total energy transferred. The average heat flow from the hot to cold bath, $\langle\dot{Q}\rangle = \gamma\kappa\langle v_x v_y\rangle$, can be calculated using Eq. (35) which reads

$$\langle\dot{Q}\rangle = k\kappa\frac{[(\alpha-1)(T_c+T_h)-2\kappa\varepsilon'^2(T_h-T_c)]\varepsilon' M+\kappa(1+\alpha-2\varepsilon'\kappa)(T_h-T_c)}{\gamma M S_0}, \tag{38}$$

and similarly the average mechanical power, $P = -\varepsilon\langle xv_y - yv_x\rangle$, can be written as

$$P = -2k\varepsilon'\frac{\kappa(1-\alpha)(T_h-T_c)+2\varepsilon'(1+\kappa^2)(T_c+T_h)}{\gamma S_0}. \tag{39}$$

The efficiency of the magneto-gyrator can be calculated and written as

$$\eta = \frac{2k\varepsilon' M[\kappa(\alpha-1)\eta_c - 2\varepsilon'(1+\kappa^2)(2-\eta_c)]}{k\varepsilon'[(\kappa(\alpha-1)-4\varepsilon'(1+\kappa^2))(2-\eta_c)-2\kappa(1-\alpha+\kappa\varepsilon'^2)\eta_c]M+\kappa^2(1+\alpha-2\varepsilon'\kappa)\eta_c} \tag{40}$$

where $\eta_c = 1 - T_c/T_h$ is the Carnot efficiency. The efficiency as a function of the diffusive Hall parameter is plotted in Fig. 5 (d) in the main text.

## References


1. Vuijk, H. D., Brader, J. M. & Sharma, A. Anomalous fluxes in overdamped Brownian dynamics with Lorentz force. *J. Stat. Mech. Theory Exp.* **2019**, 063203 (2019).

2. Chun, H.-M., Durang, X. & Noh, J. D. Emergence of nonwhite noise in Langevin dynamics with magnetic Lorentz force. *Phys. Rev. E* **97**, 032117 (2018).

3. Seifert, U. Stochastic thermodynamics, fluctuation theorems and molecular machines. *Reports on Prog. Phys.* **75**, 126001 (2012).
